# Supplementary material for: A Closer Look at Language Model Introspection: Probing Information and Reporting
Source: arXiv:2611.15267 source file (2026-11-14)
Supplement: Supplementary file 1 [file fewshot_appendix.tex]

\section{Supporting few-shot comparisons}
\label{app:fewshot}

In the base model, format-only examples that carry the same answers without any injection give \fewShotFormatOnly\% accuracy, compared with \reportBase\% without examples and \fewShotBase\% with injected examples.
The format-only improvement accounts for about half of the observed gain over zero-shot performance; this comparison does not isolate the mechanism of that improvement.
